# Supplementary material for: Stacking Characteristics of Close Packed Materials
Source: arXiv:1708.01460 source file (2017-08-04)
Supplement: Supplementary file 1 [file SM.pdf]

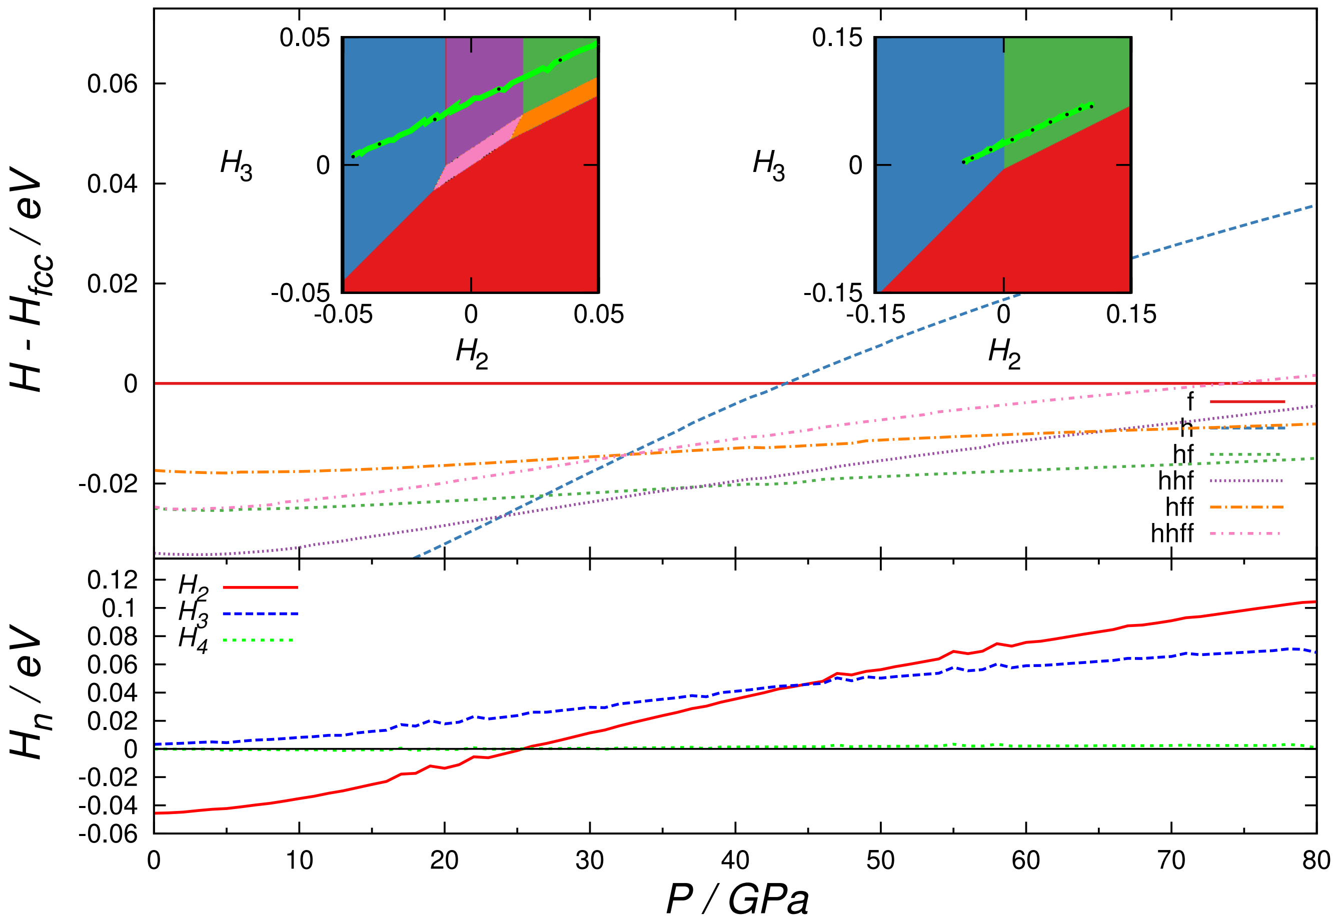


FIG. 1. DFT calculated enthalpies for phases of Scandium with pressure. (bottom) Fitted $H_n$ values with pressure. The trajectory goes through the lanthanide sequence in reverse hcp- 9R - dhcp, but experimentally it is known to transform to a complex non-close-packed structure at lower pressures than that required to reach the hcp-9R boundary The insets show the pressure-trajectory path through the ($H_2$, $H_3$, $H_4$) phase diagram projected onto planes of constant $H_4$: (left) positive $H_4$, (right) negative $H_4$. The line is green when the $H_4$ value is positive and yellow when it is negative. Small dots indicate 10 GPa intervals.

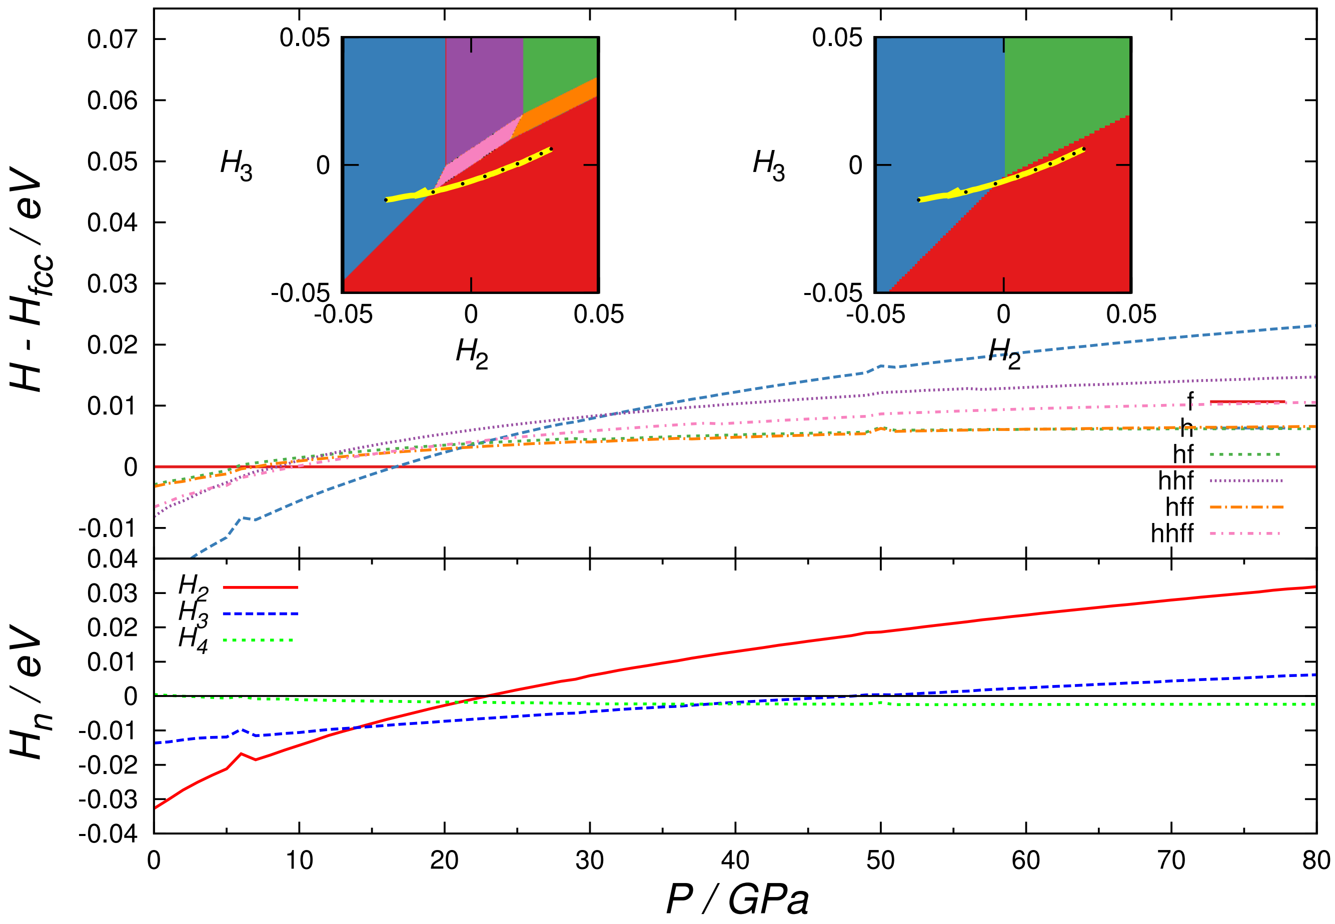


FIG. 2. DFT calculated enthalpies for phases of Thallium with pressure. (bottom) Fitted $H_n$ values with pressure. The insets show the pressure-trajectory path through the ($H_2$, $H_3$, $H_4$) phase diagram projected onto planes of constant $H_4$: (left) positive $H_4$, (right) negative $H_4$. The line pasases below the 9R and dhcp phases, indicating a direct hcp-fcc transition, as observed (Olsen et al (1994) J Appl Cryst 27:1002–1005). The line is green when the $H_4$ value is positive and yellow when it is negative. Small dots indicate 10 GPa intervals.

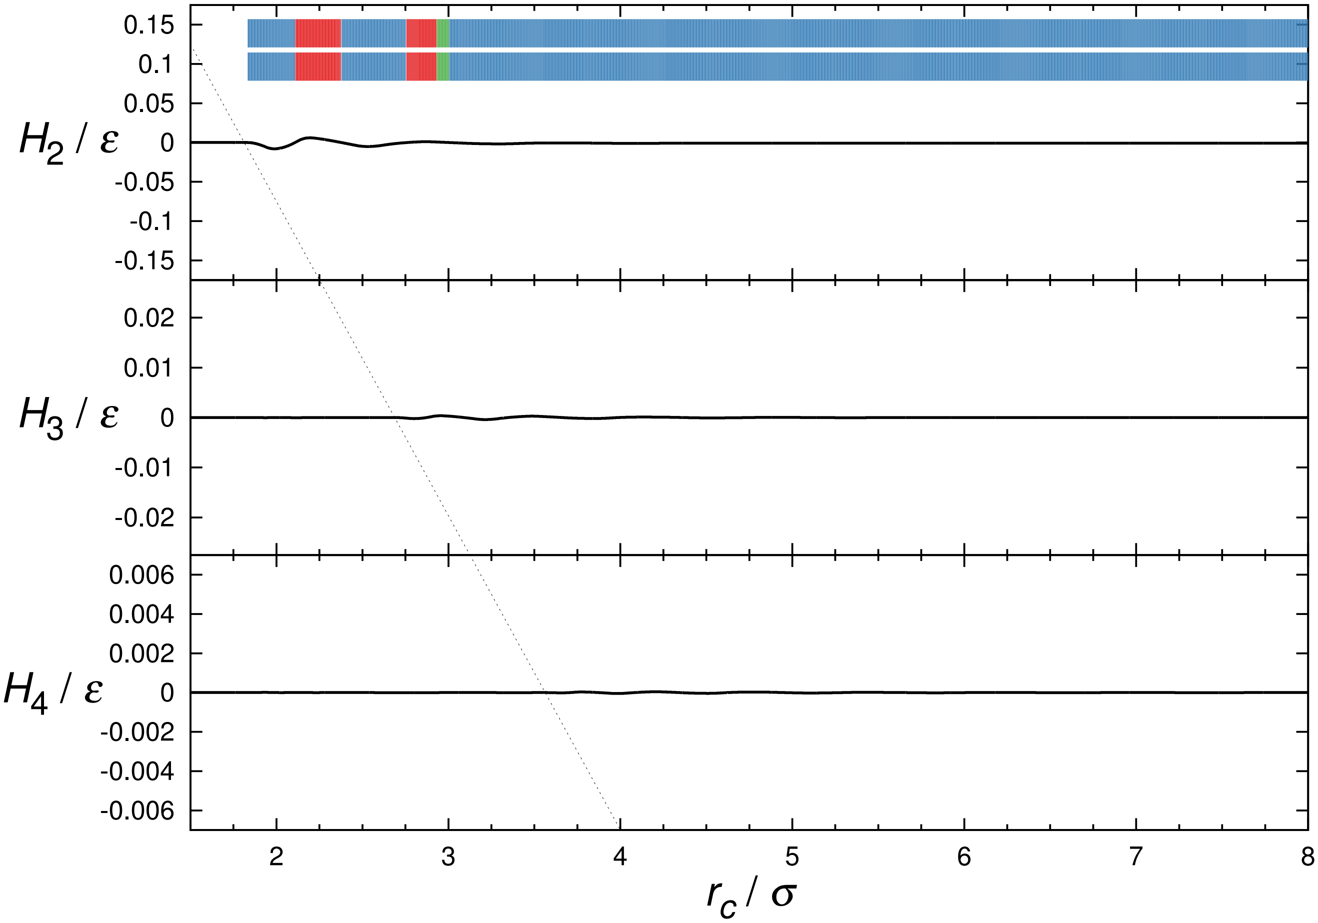


FIG. 3. Zero-pressure $H_2$, $H_3$, and $H_4$ as a function of the interaction range for the Lennard-Jones potential shifted and tilted to remove discontinuities:

$$V(r) - V(r_{cut}) + V'(r_{cut})[r_{cut} - r].$$

The diagonal dotted line demonstrates the regular introduction of new $H_i$ series at intervals of the interplanar spacing. The upper of the two ribbons at the top of the graph shows the minimum enthalpy structure at each value of the cutoff, the lower shows the minimum enthalpy structure using the $H_n$ values up to $n = 4$. The different colours represent different structures; Red: fcc, Blue: hcp, Green: dhcp.
